# Supplementary material for: VideoOrion: Tokenizing Object Dynamics in Videos
Source: arXiv:2411.16156 source file (2025-03-18)
Supplement: Supplementary file 1 [file figure-supp-case.pdf]

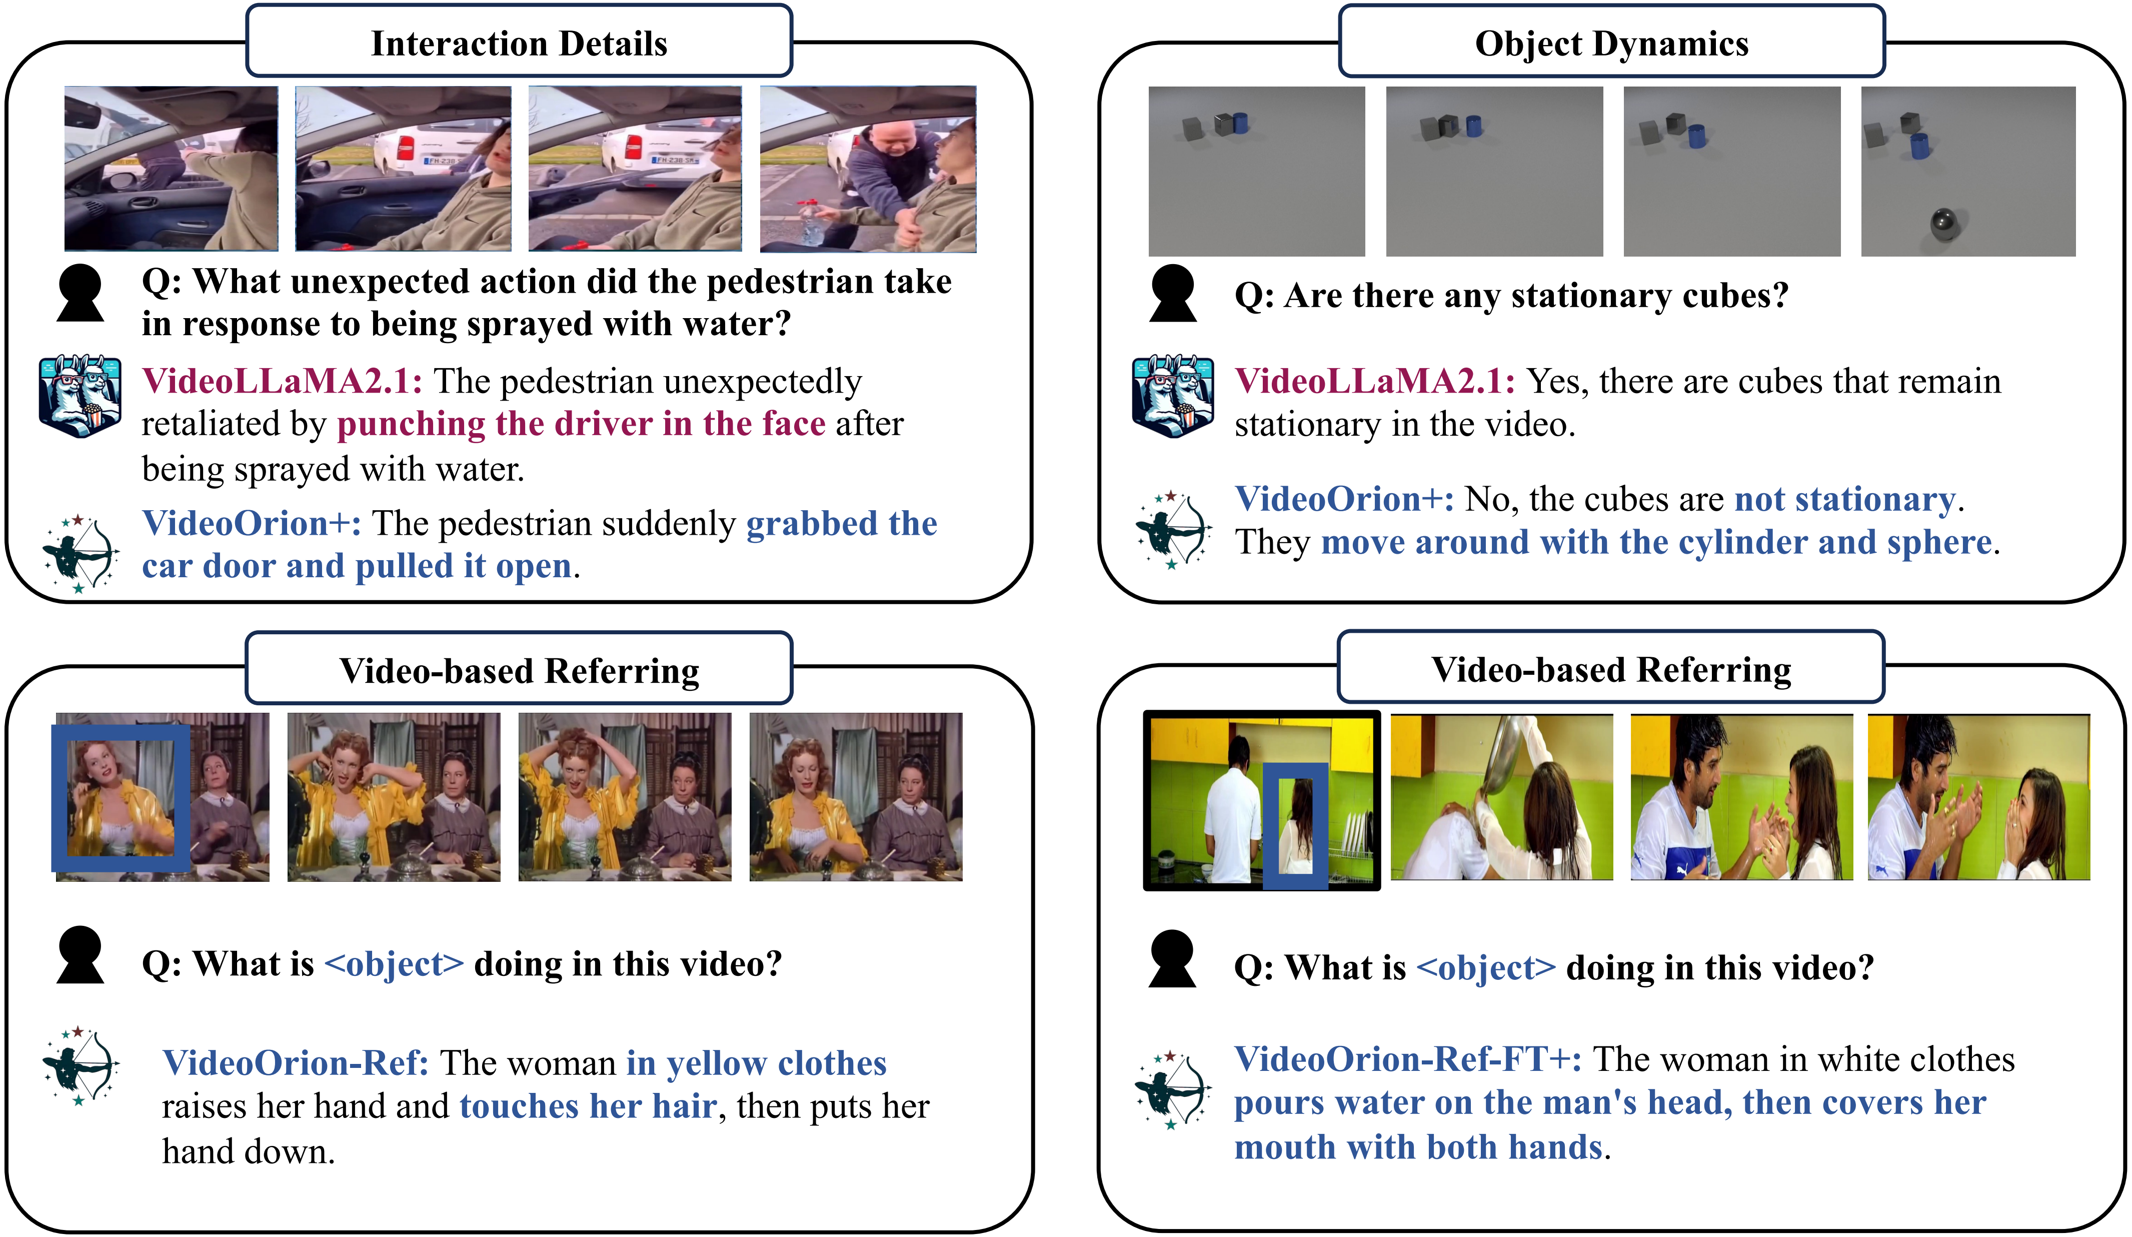
Interaction Details
Q: What unexpected action did the pedestrian take in response to being sprayed with water?
VideoLLaMA2.1: The pedestrian unexpectedly retaliated by punching the driver in the face after being sprayed with water.
VideoOrion+: The pedestrian suddenly grabbed the car door and pulled it open.
Object Dynamics
Q: Are there any stationary cubes?
VideoLLaMA2.1: Yes, there are cubes that remain stationary in the video.
VideoOrion+: No, the cubes are not stationary. They move around with the cylinder and sphere.
Video-based Referring
Q: What is <object> doing in this video?
VideoOrion-Ref: The woman in yellow clothes raises her hand and touches her hair, then puts her hand down.
Video-based Referring
Q: What is <object> doing in this video?
VideoOrion-Ref-FT+: The woman in white clothes pours water on the man's head, then covers her mouth with both hands.

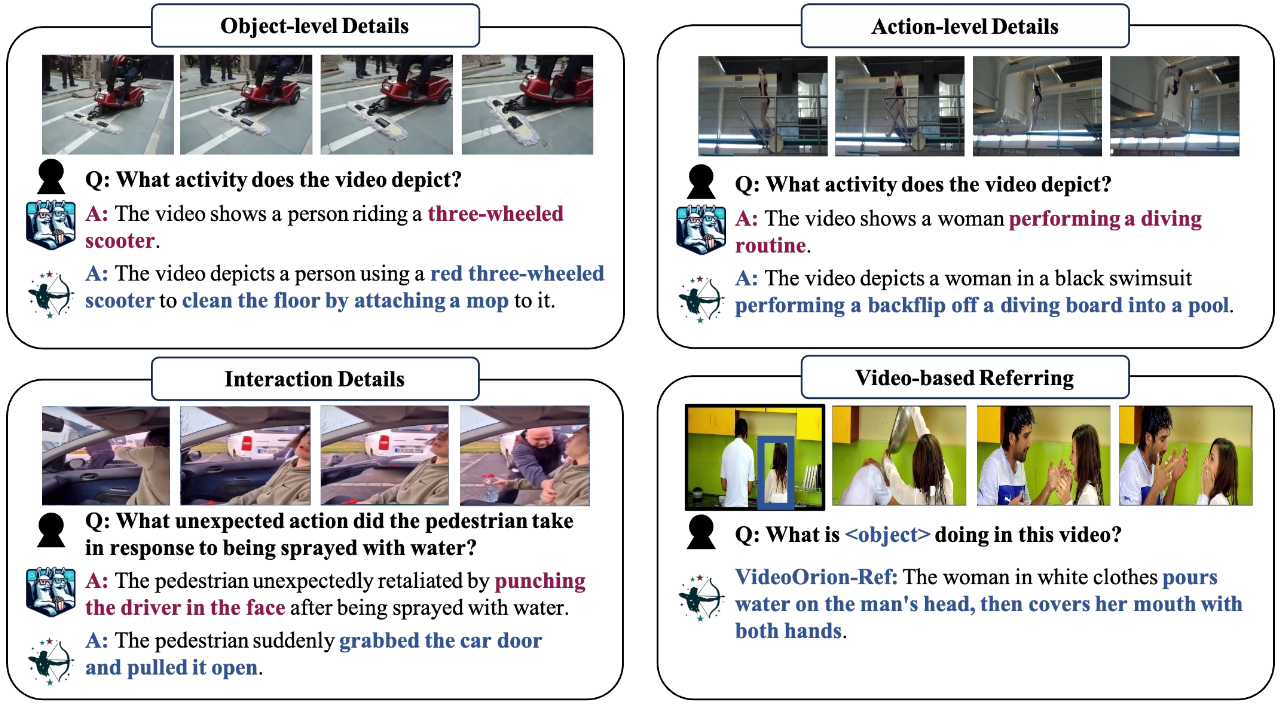
Object-level Details
Q: What activity does the video depict?
A: The video shows a person riding a three-wheeled scooter.
A: The video depicts a person using a red three-wheeled scooter to clean the floor by attaching a mop to it.
Action-level Details
Q: What activity does the video depict?
A: The video shows a woman performing a diving routine.
A: The video depicts a woman in a black swimsuit performing a backflip off a diving board into a pool.
Interaction Details
Q: What unexpected action did the pedestrian take in response to being sprayed with water?
A: The pedestrian unexpectedly retaliated by punching the driver in the face after being sprayed with water.
A: The pedestrian suddenly grabbed the car door and pulled it open.
Video-based Referring
Q: What is <object> doing in this video?
VideoOrion-Ref: The woman in white clothes pours water on the man's head, then covers her mouth with both hands.
